# Supplementary material for: Higher-twist contributions to neutrino-production of pions
Source: arXiv:1401.1547 ancillary file (2014-01-08)
Supplement: Supplementary file 1 [file Readme.pdf]

# Code for evaluation of $\nu$ DVMP cross-sections with account of twist-3 effects

This package provides a library `libDVMP` which may be used for evaluation of the  $\nu$ DVMP cross-sections with various GPD models taking into account twist-3 effects. Below are given short instructions how to compile and use it.

**Description:** This package provides a library `libDVMP` which may be used for evaluation of the  $\nu$ DVMP cross-sections in the framework discussed in the main paper. To evaluate the components of the differential cross-section, it is necessary to call the function (declared in `headers/DVMP_XSection.h`)

```
int dvmp_XSection_dlnx_dt_dQ2_dphi(
    AbstractGPD fun, double* kins,
    process p, XSection* Sigma).
```

The first argument `fun` corresponds to a GPD function declared in `headers/GPDPDF.h`, the array `kins` contains kinematic variables ordered as `kins[]={y, xB, t, Q}`, where  $y = p \cdot q / p \cdot k$ ,  $x_B$  is a Bjorken variable,  $t$  is the momentum transfer squared,  $t = \Delta^2$ ,  $Q = \sqrt{-q^2}$ . The structure `process p` declared in `headers/phys.h` contains information on particles participating in the process and has the following elements:

```
p.projectile  initial lepton ( $\nu$  or  $\bar{\nu}$ )
p.target      target ( $p$  for proton,
                  $n$  for neutron)
p.finalMeson   produced meson from
               octet of pseudogoldstones
               ( $\pi^{0,\pm}$ ,  $K_{L,S}$ ,  $K^\pm$  or  $\eta$ )
p.finalBaryon  produced baryon from
               lowest octet ( $p$ ,  $n$ ,  $\Lambda$ ,  $\Sigma^{0,\pm}$ )
p.finalLepton  produced lepton ( $\nu$ ,  $\bar{\nu}$ ,  $\mu^\pm$ )
```

If evaluation was successful, `SUCCESS` value is returned and elements of `Sigma` are set to the components of the unintegrated cross-section  $x_B d^4\sigma_k / dt dx_B dQ^2 d\phi$  according to the following table:

|                            |                                                  |
|----------------------------|--------------------------------------------------|
| <code>Sigma.L</code>       | $\frac{d^4\sigma_L}{dt d\ln x_B dQ^2 d\phi}$     |
| <code>Sigma.T</code>       | $\frac{d^4\sigma_T}{dt d\ln x_B dQ^2 d\phi}$     |
| <code>Sigma.LT</code>      | $\frac{d^4\sigma_{LT}}{dt d\ln x_B dQ^2 d\phi}$  |
| <code>Sigma.TT</code>      | $\frac{d^4\sigma_{TT}}{dt d\ln x_B dQ^2 d\phi}$  |
| <code>Sigma.LPrimeT</code> | $\frac{d^4\sigma_{L'T}}{dt d\ln x_B dQ^2 d\phi}$ |
| <code>Sigma.TPrimeT</code> | $\frac{d^4\sigma_{T'T}}{dt d\ln x_B dQ^2 d\phi}$ |
| <code>Sigma.H.c[n]</code>  | $c_n$ -harmonics ( $n = 0, 1, 2$ )               |
| <code>Sigma.H.s[n]</code>  | $s_n$ -harmonics ( $n = 1, 2$ )                  |

Other possible return values are `PROCESS_NOT_FOUND` if process is unknown and `WRONG_KINEMATICS` if the cross-section in unphysical kinematics is called. In both cases components of `Sigma` are undefined.

The GPD models needed for numerical evaluations are placed in separate library files in folder `libraries/`. With this package, we provide the Kroll-Goloskokov [1] GPD model (file `libKrollGoloskokovGPD11.so`) described in the text of the paper.

**Prerequisites:** To compile this code, You need to have `C` and `Fortran 77` compilers, `make` utility and a GNU scientific library (GSL) installed. The code was tested with `gcc v. 4.4` and `4.6` and `Fortran compiler gfortran` on Linux `x86-64` platform.

**Compilation:** To compile the code, You have to run `make` all in the code main directory. This will build the above-mentioned GPD library, the  $\nu$ DVMP library (`libDVMP.so`, `libDVMP.a`) and an example driving application `NuDVMP` (see source in `src/DVMP.c`) which shows how to load GPDs from corresponding libraries and evaluate the cross-section.

**Running:** After compilation, run from command-line `./NuDVMP --NeutrinoType NuMuBar --Target Proton --Lepton MuPlus --Meson PiZero --DeltaTr 0.2 --Baryon Neutron --lepton-fraction 0.5 --virtuality 2 --gpd-model libraries/libKrollGoloskokovGPD11.so` or in a brief form <sup>1</sup>

```
./NuDVMP -N NuMuBar -T Proton -L MuPlus
-M PiZero -B Neutron -y 0.5 -q 2 -d 0.2 -g
libraries/libKrollGoloskokovGPD11.so
```

This will evaluate the cross-section  $x_B d^4\sigma / dt dx_B dQ^2 d\phi$  for the process  $\bar{\nu}p \rightarrow \mu^+\pi^0n$  as a function of  $x_B$  at virtuality  $Q = 2$  GeV and  $y = 0.5$ , with  $\Delta_\perp = 0.2$  GeV and using Kroll- Goloskokov GPD model. Optionally, instead of fixed  $\Delta_\perp$ , one can make evaluations at fixed  $t$  with `-t` option. If only leading twist results are needed, evaluations may be done faster with option `--use-twist3 no` or `-w n`. For other possible options, run `./NuDVMP --help`.

**Adding new GPD models:** In order to add a new GPD model, You have to implement a function `ExternalGPD(double x, struct GPDKins k)`, where  $x$  is the quark light-cone fraction and `struct GPDKins` declared in `headers/GPDPDF.h` keeps all the information on the target kinematics and has the following elements:

```
k.xi          skewness parameter  $\xi$ 
k.t            momentum transfer  $t = \Delta^2$ 
k.Q            Scale at which GPD is taken
k.flavour      GPD flavour
k.GPD_type     Type of GPD, can be
                GPD_H ( $H$ ), GPD_E ( $E$ ), GPD_HTilde ( $\tilde{H}$ )
                GPD_ETilde ( $\tilde{E}$ ), GPDT_H ( $H_T$ ), GPDT_E ( $E_T$ ),
                GPDT_HTilde ( $\tilde{H}_T$ ), GPDT_ETilde ( $\tilde{E}_T$ ).
```

<sup>1</sup> Optionally, instead of particle names, PDG codes of the particles can be used; only particles and processes mentioned in the text of the paper are supported.

After successful compilation of the the new GPD model `libNewGPD.so`, it can be used with `--gpd-model` option discussed above, without recompilation of other parts of the code. For more details, please see the header files in

`headers/` directory. Each function has a Doxygen-style comments with detailed description. Corresponding `.c`-files are in `src/` directory.

- 
- [1] S. V. Goloskokov and P. Kroll, Eur. Phys. J. A **47**, 112 (2011) [arXiv:1106.4897 [hep-ph]].
