# Supplementary material for: Higher-twist contributions to neutrino-production of pions
Source: arXiv:1401.1547 ancillary file (2014-01-08)
Supplement: Supplementary file 2 [file pfq.pdf]

# A NUMERICAL EVALUATOR FOR THE GENERALIZED HYPERGEOMETRIC SERIES<sup>†</sup>

WARREN F. PERGER\*, ATUL BHALLA\*\*, AND MARK NARDIN\*\*\*

*\*Electrical Engineering Department and Physics Department, Michigan Technological University, Houghton, MI 49931, USA*

**\*\*Verilink Corporation, 145 Baytech Drive, San Jose, CA 95134, USA**

\*\*\**Electrical Engineering Department, University of Michigan, Ann Arbor, MI*

<sup>†</sup>*This work supported in part by a grant from the National Science Foundation, CCR-8823031.*

Received: \_\_\_\_\_; in revised form: \_\_\_\_\_

## Abstract

The generalized hypergeometric series is numerically evaluated using extended precision subroutines. Cases involving large, complex arguments are shown to be accurate up to 12 significant figures.

## PROGRAM SUMMARY

*Title of program:* PFQ

*Catalogue number:*

*Program obtainable from:* CPC Program Library, Queen's University of Belfast, N. Ireland  
(see application form in this issue)

*Licensing provisions:* none

*Computer for which the program is designed and others on which it has been tested:*

*Computers:* Sun SPARC Station, IBM 4381, IBM RS6000;

*Installations:* Michigan Technological University;

*Operating systems or monitors under which the program has been tested:*

Sun OS 4.1.1, 4.1.2; IBM CMS VM/SP HOP 5.0; IBM AIX 3.1.5;

*Programming language used in the program:* FORTRAN 77

*Memory required to execute with typical data:* 16 million (8 bit) words

*No. of bits in a word:* 8

*Number of processors:* 1

*Has the code been vectorised?* No.

*No. of lines in distributed program, including test data, etc.:* 1721

*Additional Keywords:* special functions, confluent hypergeometric function

*Nature of physical problem* The generalized hypergeometric series is the solution of many equations occurring in various scientific and engineering disciplines. A couple of examples are: the radial part of the wavefunction of the hydrogen atom, for bound and continuum states both non-relativistic and relativistic, and the radial and angular parts of the solution to the biconical antenna.

*Method of solution* The generalized hypergeometric series is summed using extended precision complex arrays.

*Restrictions on the complexity of the problem* The program is fundamentally limited by the amount of available memory. A PARAMETER statement sets the variable LENGTH, which is the maximum size of any of the extended precision arrays (the distributed version of PFQ has LENGTH=777).

*Typical running time* The running time may vary widely, on a given machine, depending on the number of terms required in the summation to achieve convergence. On a Sun SPARCStation 1, the time required has been observed to be as small as 1 second and as large as 20 minutes.

*Unusual features of the program* The program automatically estimates the number of bits available in the mantissa and sets the number of array positions required accordingly. The program also scans the input data looking for input parameters that would result in a division by zero or a finite series. In either case, the program examines the incoming parameter(s), comparing them against zero, considering the number of bits available in the mantissa. If a number is close enough to zero to meet this criterion, the program prints a message to the user and either continues or aborts, depending on the anticipated impact. The user options include the ability to request a specific number of significant figures in the result, whether or not to return the result in natural logarithm form, and the ability to manually or automatically determine the number of array elements to be used in the extended arithmetic.

# LONG WRITE-UP

## 1. Introduction

### 1.1. Details of Solution

The generalized hypergeometric series  ${}_pF_q[(\alpha)_p; (\beta)_q; z]$  satisfies the differential equation[1]:

$$\left\{ z \frac{d}{dz} \left( z \frac{d}{dz} + \beta_1 - 1 \right) \left( z \frac{d}{dz} + \beta_2 - 1 \right) \cdots \left( z \frac{d}{dz} + \beta_q - 1 \right) - \right. \quad (1)$$

$$\left. z \left( z \frac{d}{dz} + \alpha_1 \right) \left( z \frac{d}{dz} + \alpha_2 \right) \cdots \left( z \frac{d}{dz} + \alpha_p \right) \right\} {}_pF_q[(\alpha)_p; (\beta)_q; z] = 0, \quad (2)$$

where

$$\begin{aligned} {}_pF_q[(\alpha)_p; (\beta)_q; z] &= 1 + \frac{\alpha_1 \alpha_2 \cdots \alpha_p z}{\beta_1 \beta_2 \cdots \beta_q 1!} + \frac{\alpha_1(\alpha_1 + 1) \alpha_2(\alpha_2 + 1) \cdots \alpha_p(\alpha_p + 1) z^2}{\beta_1(\beta_1 + 1) \beta_2(\beta_2 + 1) \cdots \beta_q(\beta_q + 1) 2!} + \cdots \\ &= \sum_{n=0}^{\infty} \frac{(\alpha_1)_n (\alpha_2)_n \cdots (\alpha_p)_n z^n}{(\beta_1)_n (\beta_2)_n \cdots (\beta_q)_n n!}. \end{aligned} \quad (3)$$

The symbol used in (3), the Pochhammer symbol, is defined as:

$$(\alpha_1)_n = \alpha_1(\alpha_1 + 1) \cdots (\alpha_1 + n - 1). \quad (4)$$

Consequently, Equation (2) fits a rather broad class of problems which are commonly encountered in various scientific disciplines. When  $p=1$  and  $q=1$ , (3) becomes the confluent hypergeometric function, which includes Bessel, Coulomb Wave, Laguerre, etc., functions [2, page 509]. When  $p=2$  and  $q=1$ , the  ${}_2F_1$  series (commonly referred to as the Gauss hypergeometric series) results, which has Chebyshev, Legendre, and Jacobi polynomials as examples of special cases[2, page 561]. The program described in this paper is a numerical evaluator of the series of Equation (3) and will converge under the conditions that the series converges. The only transformation formula employed is the use of the linear transformation 15.3.6 of Abramowitz and Stegun[2] for the case where  $p=2$ ,  $q=1$ , and  $|z|$  is approaching 1 from below. Because the program uses arrays to achieve extended precision complex arithmetic, the size of the partial sum (and therefore the final answer) will depend on the available memory. However, on a Sun SPARCStation 1 with 28MByte of memory, convergence was attained for cases involving 60,000 terms.

The method of summing the series using extended precision arrays follows closely the predecessor to this program, CONHYP, written for the confluent hypergeometric function[3]. Additionally, the tests employed to verify the accuracy of the current program were similar to those described by Nardin, et al [4]. Therefore, in this paper, only the significant differences in the program [3] and the testing procedure [4] will be described.

## 2. Program Structure

### 2.1. Function *PFQ*

The evaluation of the series in (3) is accomplished by a function call to *PFQ*, which is a double precision complex function. The required input is:

1. Double precision complex arrays *A* and *B*. These are the arrays containing the parameters in the numerator and denominator, respectively.
2. Integers *IP* and *IQ*. These integers indicate the number of numerator and denominator terms, respectively (these are *p* and *q* in (3)).
3. Double precision complex argument *Z*.
4. Integer *LNPFQ*. This integer should be set to “1” if the result from *PFQ* is to be returned as the natural logarithm of the series, or “0” if not. The user can generally set *LNPFQ* = “0” and change it if required.
5. Integer *IX*. This integer should be set to “0” if the user desires the program *PFQ* to estimate the number of array terms (in *A* and *B*) to be used, or an integer greater than zero specifying the number of integer positions to be used. This input parameter is especially useful as a means to check the results of a given run. Specifically, if the user obtains a result for a given set of parameters, then changes *IX* and re-runs the evaluator, and if the number of array positions was insufficient, then the two results will likely differ. The recommended procedure would be to generally set *IX* = “0” and then set it to 100 or so for a second run. Note that the *LENGTH* parameter currently sets the upper limit on *IX* to 777, but that can easily be changed (it is a single *PARAMETER* statement) and the program recompiled.
6. Integer *NSIGFIG*. This integer specifies the requested number of significant figures in the final result. If the user attempts to request more than the number of bits in the mantissa allows, the program will abort with an appropriate error message. The recommended value is 10.

### 2.2. Function *BITS*

*BITS* determines the number of significant figures in the mantissa.

### 2.3. Function *HYPER*

*HYPER* screens the incoming parameters looking for incorrect or inappropriate data, then calls the various subprograms to sum the series in (3).

### 2.4. Subroutines *ARADD*, *ARSUB*, *ARMULT*, *ARYDIV*

These subroutines add, subtract, multiply, and divide two double precision arrays, respectively, and return the appropriate result.

### 2.5. Subroutines *CMPADD*, *CMPSUB*, *CMPMUL*

These subroutines add, subtract, and multiply, respectively two double precision complex arrays.

### 2.6. Subroutines *EADD*, *ESUB*, *EMULT*, *EDIV*

These subroutines add, subtract, multiply, and divide, respectively, two double precision complex numbers mantissa and exponent and return the appropriate mantissa and exponent.

### 2.7. Subroutines *CONV12* and *CONV21*

These subroutines convert a double precision complex number to the form of a 2x2 array, and vice-versa, respectively.

### 2.8. Subroutines *IPREMAX* and *FACTOR*

These subroutines are used to predict the maximum exponent required in the summation given in (3). This estimate is then used to set the number of array positions required for the successful summation of the series.

## 3. Description of test data

The test data is in the form of a FORTRAN “driver” program which calls PFQ and compares the result for the case of  ${}_1F_1$ . The computer used for this test case was a Sun SPARCStation 1, running SunOS 4.1.2, with 28MByte of memory. This particular case ran roughly three times faster using PFQ than Mathematica<sup>®</sup>.

This driver program will be given here for completeness:

```
PROGRAM SAMPLE
COMPLEX*16 P,Q,Z,PFQ,RESULT
INTEGER LNPFQ,IP,IQ,IX,NSIGFIG
DIMENSION P(10),Q(10)
DOUBLE PRECISION AR,AI
*
OPEN (5,FILE='DATA',STATUS='OLD')
READ (5,*) IP,IQ
DO 1 I=1,IP
  READ (5,*) P(I)
  WRITE (6,*) ' P(I)= ',P(I)
1 CONTINUE
DO 2 I=1,IQ
  READ (5,*) Q(I)
  WRITE (6,*) ' Q(I)= ',Q(I)
```

```

2 CONTINUE
  READ (5,*) Z
  WRITE (6,*) ' Z= ',Z
  READ (5,*) LNPFQ
  WRITE (6,*) ' LNPFQ= ',LNPFQ
  READ (5,*) IX
  WRITE (6,*) ' IX= ',IX
  READ (5,*) NSIGFIG
  WRITE (6,*) ' NSIGFIG= ',NSIGFIG
  RESULT = PFQ(P,Q,IP,IQ,Z,LNPFQ,IX,NSIGFIG)
  WRITE (6,300)
  WRITE (6,301) RESULT
  AR=2.31145634403D-12
  AI=-1.96169649635D-11
  WRITE (6,302) AR,AI
300 FORMAT (32X,'REAL PART',16X,'IMAG PART')
301 FORMAT (1X,' RESULT FROM PFQ=',3X,1P,2D25.11)
302 FORMAT (1X,' EXPECTED RESULT=',3X,1P,2D25.11)
  STOP
  END

```

## Acknowledgments

The authors gratefully acknowledge the comments of Dr. Jim Cody which contributed significantly to the predecessor to this program. We also wish to thank the referee for pointing out several weaknesses which we have now taken into account and which will undoubtedly improve the program.

## References

- [1] L. J. Slater, *Generalized Hypergeometric Functions*, Cambridge University Press, Cambridge, England, 1966.
- [2] M. Abramowitz and I. A. Stegun, *Handbook of Mathematical Functions*, Dover Publications, New York, 1970.
- [3] M. Nardin, W. F. Perger, and A. Bhalla, ACM Trans. Math. Softw. **18** (1992) 345.
- [4] M. Nardin, W. F. Perger, and A. Bhalla, J. Comput. Appl. Math. **39** (1992) 193.



## TEST RUN INPUT

```
1 1
(-15.0D0,55.0D0)
(20.0D0,25.0d0)
(-100.0D0,200.0D0)
0
0
10
```

## TEST RUN OUTPUT

P(I)= ( -15.0000000000000, 55.0000000000000)

Q(I)= ( 20.0000000000000, 25.0000000000000)

Z= ( -100.0000000000000, 200.0000000000000)

LNPFQ= 0

IX= 0

NSIGFIG= 12

|                  | REAL PART         | IMAG PART          |
|------------------|-------------------|--------------------|
| RESULT FROM PFQ= | 2.31145634403D-12 | -1.96169649635D-11 |
| EXPECTED RESULT= | 2.31145634403D-12 | -1.96169649635D-11 |
